# Supplementary material for: Fixed-Point Approaches to Computing Bertrand-Nash Equilibrium Prices Under Mixed Logit Demand: A Technical Framework for Analysis and Efficient Computational Methods
Source: arXiv:1012.5836 source file (2010-12-28)
Supplement: Supplementary file 1 [file additionaldetails.tex]

\section{Additional Details Regarding the Numerical Examples}
\label{ECSEC:AdditionalDetails}

	%%%%%%%%%%%%%%%%%%%%%%%%%%%%%%%%%%%%%%%%%%%%%%%
	%%%%%%%%%%%%%%%%%%%%%%%%%%%%%%%%%%%%%%%%%%%%%%%
	%%%%%%%%%%%%%%%%%%%%%%%%%%%%%%%%%%%%%%%%%%%%%%%
	
	\subsection{The Two Demand Models}
	\label{ECSUBSEC:DemandModels}
	
	To characterize demand for new vehicles, we employ modified versions of two existing models of new vehicle purchasing \citep{Boyd80,Berry95}. Here we give a brief description of the versions of these models used in our examples below. Random coefficient distributions are described by the parameters given in Tables \ref{TAB:BM80Coeffs} and \ref{TAB:BLP95Coeffs}. 
	
	The utility function in the \cite{Boyd80} model is linear in characteristics and price with lognormally distributed ``unobserved'' demographic variables (random coefficients) $\bsym{\theta}$, has no ``observed'' demographic variables, and does not model an outside good (i.e., $\vartheta(\bsym{\theta}) \equiv -\infty$). Specifically, with $\bsym{\theta} = (\alpha,\bsym{\beta}) \in \set{P} \times \R^3$, 
	 \begin{equation*}
	 	u(\alpha,\bsym{\beta},\vec{x},p) 
			= - \alpha p + \bsym{\beta}^\top\vec{x}
			= - \alpha p + \beta_1 x_1 + \beta_2 x_2 - \beta_3 x_3
	 \end{equation*}
	 We include the vehicle characteristics 
	 \begin{itemize}
	 	\item $x_1$: ``size'' (length times width over height, all in inches),
		\item $x_2$: ``acceleration'' (60 divided by the 0-60 acceleration time, in seconds), and 
		\item $x_3$: ``fuel consumption'' (100 times fuel consumption, in gallons per mile). 
	\end{itemize}
	A simple function of horsepower to weight ratio approximates 0-60 acceleration, a commonly used proxy in econometric models of the vehicle market. Due to a lack of data, we exclude several consumer reports ratings (``ride,'' ``handling,'' and ``noise'') used in the original model. We use 1980 USD as our monetary units. 
	
	The utility function in the \cite{Berry95} model is linear in characteristics with independent and normally distributed ``unobserved'' demographics (random coefficients), nonlinear in income minus price, and models an outside good. Specifically, with $\bsym{\theta} = (\phi,\bsym{\beta},\beta_0) \in \set{P} \times \R^3 \times \R$, 
	 \begin{equation*}
	 	% \label{BLPTypeUtility}
	 		u(\phi,\bsym{\beta},\beta_0,\vec{x},p) 
				= \alpha \log( \phi - p ) + \bsym{\beta}^\top\vec{x}
			\quad\quad\text{and}\quad\quad
			\vartheta(\phi,\bsym{\psi},\nu) = \alpha \log \phi + \beta_0
	 \end{equation*}
	 for a price coefficient $\alpha = 43.501 > 1$, income $\phi$, and random coefficients $\bsym{\beta}$. Consistent with the original model, we take income, price, and cost to be in thousands of 1983 USD where income is lognormally distributed with a log-mean of $10 - 3 \log 10 \approx 3.092$ and a log-standard deviation of 1 \citep{CPS05}. For vehicle characteristics we include 
	 \begin{itemize}
	 	\item $x_1$: operating cost (in 10 mile increments driven per dollar spent using a fuel price of 2.50 2005 USD = 1.27 1983 USD), 
		\item $x_2$: horsepower to weight ratio (weight is in 10 lbs.), and 
		\item $x_3$ length times width (both in hundreds of inches). 
	\end{itemize}
	We effectively exclude a dummy variable for standard air conditioning present in the original model by assuming standard air conditioning on all vehicles (the utility value for this is absorbed into the utility of the outside good). No other characteristics from the original model differ in our version. The random coefficients $\bsym{\beta}$ and $\beta_0$ are independently normally distributed with means and standard deviations listed in Table \ref{TAB:BLP95Coeffs}. 
	 
	 \begin{table}
	 	\TABLE
		{Coefficients describing the (lognormal) distribution of the random coefficients Mixed Logit model estimated by \cite{Boyd80}. \label{ECTAB:BM80Coeffs}}
	 	{\begin{tabular}{rcccc}
						& $\alpha$ & $\beta_1$ 	& $\beta_2$ 	& $\beta_3$	\\ \hline
			log-mean		& -7.96	& 0.589		& -1.75		& -1.28 		\\
			log-std. dev. 	& 1.18	& 0.622		& 1.34		& 0.001		\\ \hline
			\\
		\end{tabular}}
		{}
	\end{table}
	
	 \begin{table}
	 	\TABLE
		{Coefficients describing the (normal) distribution of the random coefficients Mixed Logit model estimated by \cite{Berry95}. $\phi$ is lognormally distributed, and thus reported values are the log-mean and log-standard deviation. \label{ECTAB:BLP95Coeffs}}
		{\begin{tabular}{rcccccc}
					& $\alpha$ 	& $\phi$ 	& $\beta_1$ 	& $\beta_2$ 	& $\beta_3$	& $\beta_0$ \\ \hline
			mean	& 43.501		& 10		& -0.122		& 3.460		& 2.883		& -8.582 \\
			std. dev.	& $-$		& 1		& 1.05		& 2.056		& 4.628		& 1.794 \\ \hline
		\end{tabular}}
		{}
	\end{table}

	 \begin{proposition}
	 	\label{BMandBLPFunctions} 
		\begin{itemize}
			\item[(i)] Assumption \ref{MixedLogitUtilityAssump} holds for both the \cite{Boyd80} and \cite{Berry95} models. 
			\item[(ii)] The conclusions of Proposition \ref{LeibnizRule} hold under the \cite{Boyd80} model. Assumption \ref{LeibnizRuleCondition}, and hence the conclusions of Proposition \ref{LeibnizRule}, hold under the \cite{Berry95} model so long as $\alpha > 1$. 
		\end{itemize}
	 \end{proposition}
	 \begin{remark}
	 We treat the \citeauthor{Boyd80} model separately because it does not have an outside good, and hence does not match the format of Assumption \ref{LeibnizRuleCondition}. The requirement that $\alpha > 1$ under the \citeauthor{Berry95} model ensures the continuously differentiability of $P_j^L(\phi,\bsym{\beta},\vec{p})$ at $p_j = \phi$. 
	 \end{remark}
	 
	\proof{Proof:}
		
		The \cite{Boyd80} model takes 
		\begin{align*}
		 	w(\alpha,\bsym{\beta},\vec{x},p) 	
				= - \alpha p
			\quad \quad\text{and}\quad \quad
			v(\alpha,\bsym{\beta},\vec{x}) 	
				= \bsym{\beta}^\top\vec{x}
		 \end{align*}
		 with no outside good. As mentioned above, $\abs{(D_kP_j^L)(\bsym{\theta},\vec{p})} \leq \abs{(Dw_k)(\bsym{\theta},p_k) }$ always holds. While this is not useful in general, it can be applied here to derive $\abs{(D_kP_j^L)(\alpha,\bsym{\beta},\vec{p})} \leq \alpha$, a bound that demonstrates the uniform $\mu$-integrability of the choice probability derivatives for any probability measure $\mu$ giving a finite expected price coefficient. Thus the conclusions of Proposition \ref{LeibnizRule} hold, since there is a finite expected price coefficient under the \citeauthor{Boyd80} model. 
	
		The \cite{Berry95} model takes $\bsym{\theta} = (\phi,\bsym{\beta},\beta_0)$ and
		\begin{align*}
		 	w(\phi,\bsym{\beta},\beta_0,\vec{x},p) 		
				= \alpha \log( \phi - p ), 
			\quad\quad
			v(\phi,\bsym{\beta},\beta_0,\vec{x},p) 
				= \bsym{\beta}^\top\vec{x},
			\quad\quad\text{and}\quad\quad
			\vartheta(\phi,\bsym{\beta},\beta_0) 
				= \alpha \log( \phi ) + \beta_0. 
		\end{align*}
		The hypothesis of Proposition \ref{LeibnizRule} is not satisfied if $\alpha < 1$: For all $\phi > p$, we have
		\begin{align*}
		 	\abs{(Dw)(\bsym{\theta},\vec{x},p)} e^{ u(\bsym{\theta},\vec{x},p) - \vartheta(\bsym{\theta}) }
			 	&= \alpha \left( \frac{1}{\phi} \right)^\alpha \left( \frac{1}{\phi-p} \right)^{1-\alpha} e^{\bsym{\beta}^\top\vec{x} - \beta_0}
		\end{align*}
		which is not $\mu$-integrable at $\phi = p$, for any $p > 0$, for any probability measure $\mu$ supported on a subset of $[0,\infty)$. By assuming $\alpha > 1$ we have instead
		\begin{align*}
		 	\abs{(Dw)(\bsym{\theta},\vec{x},p)} e^{ u(\bsym{\theta},\vec{x},p) - \vartheta(\bsym{\theta}) }
			 	&= \alpha \left( \frac{1}{\phi} \right)^\alpha \left( \phi - p \right)^{\alpha-1} e^{\bsym{\beta}^\top\vec{x} - \beta_0}
		\end{align*}
		which $\mu$-integrable for any probability measure $\mu$ supported on a subset of $[0,\infty)$. 
		
		In addition, $\abs{(Dw)(\bsym{\theta},\vec{x},p)} e^{ u(\bsym{\theta},\vec{x},p) - \vartheta(\bsym{\theta}) }$ vanishes as $\phi \downarrow p$. Thus we set 
		\begin{align*}
		 	\abs{(Dw)(\bsym{\theta},\vec{y},p)} e^{ u(\bsym{\theta},\vec{x},p) - \vartheta(\bsym{\theta}) }
				= \varphi_p(\phi)e^{\bsym{\beta}^\top\vec{x} - \beta_0}
		\end{align*}
		where now
		\begin{align*}
		 	\varphi_p(\phi)
				= \left\{ \begin{aligned}
					&\alpha \left( \frac{(\phi - p)^{\alpha - 1}}{\phi^\alpha} \right)
						&&\quad\text{if } \phi > p \\
					&\quad\quad\;\; 0 &&\quad\text{if } \phi \leq p
				\end{aligned} \right.
		\end{align*}
		We can take $\mu = \mu_\phi \times \mu_\beta$ where $\mu_p$ is a measure for $\phi$ giving it a lognormal distribution and $\mu_\beta$ is a measure for $(\bsym{\beta},\beta_0)$ giving it a normal distribution. By Fubini's theorem, 
		 \begin{align*}
		 	&\int \abs{(Dw)(\bsym{\theta},\vec{x},p)} e^{ u(\bsym{\theta},\vec{x},p) - \vartheta(\bsym{\theta}) } d\mu(\bsym{\theta}) \\
			&\quad\quad
				= \int \int \varphi_p(\phi) d\mu_\phi(\phi) \; e^{\bsym{\beta}^\top\vec{x} - \beta_0} d\mu_\beta(\bsym{\beta},\beta_0) \\
			&\quad\quad
				= \left( \int e^{\bsym{\beta}^\top\vec{x} - \beta_0} d\mu_\beta(\bsym{\beta},\beta_0) \right)
					\int \varphi_p(\phi) d\mu_\phi(\phi)
		\end{align*}
		The normal distribution on $(\bsym{\beta},\beta_0)$ ensures that
		\begin{align*}
		 	\int e^{\bsym{\beta}^\top\vec{x} - \beta_0} d\mu_\beta(\bsym{\beta},\beta_0) < \infty. 
		\end{align*}
		We turn to the price term, $\int \varphi_p(\phi) d\mu_p(\phi)$. If $p \leq p^\prime$, then $\varphi_p(\phi) \geq \varphi_{p^\prime}(\phi)$ for all $\phi$. Thus, $\varphi_p(\phi) \leq \varphi_0(\phi)$ for all $\phi$ and any $p > 0$. Now $\varphi_0(\phi) = \alpha \phi^{\alpha - 2}$, an integrable function with respect to the measure $\mu_p$ for any $\alpha > 1$. Hence $\abs{(Dw)(\bsym{\theta},\vec{y},p)} e^{ u(\bsym{\theta},\vec{y},p) - \vartheta(\bsym{\theta}) } $ is uniformly $\mu$-integrable in a neighborhood of $p$, for any $p > 0$. \Halmos
		
	\endproof
	
	\subsection{Extrapolation of Costs}
	\label{ECSUBSEC:Extrapolation}
	
	Section \ref{SUBSEC:Sensitivity} considers a differentiated product market model with 5,298 vehicles derived from the Ward's data. To generate this larger problem we extrapolate the J. D. Power cost data by assuming that variation in dealer costs is reflected in the MSRP reported by Ward's. Specifically, we define a model-year plus trim's dealer cost as the average dealer cost for the model-year vehicle with which it is associated plus the deviation of the model-year variant specific MSRP from the average MSRP across all variants of that model-year. 
	 
	\subsection{``Arbitrary'' Initial Conditions}
	\label{ECSUBSEC:InitialConditions}
	
	Our ``arbitrary'' initial conditions used in Section \ref{SUBSEC:Sensitivity} were formally defined as follows. For the \citeauthor{Boyd80} model initial conditions are drawn uniformly from $[ \min_{j \in \N(J)} c_j , \max_{j \in \N(J)} c_j ]^J$. For the \citeauthor{Berry95} model, the finite reservation price (income) makes choosing arbitrary initial conditions more difficult. We draw initial conditions uniformly from $[0,19000]^J$, where the $70\ith$ percentile of income is approximately $19,000$ 1983 USD. Using this upper limit ensures that, loosely speaking, the upper 30 \% of the sampled population can buy {\em any} vehicle at the initial prices, and does {\em not} preclude the existence of individuals in the sampled population that have an income too low to buy any of the vehicles at their initial prices. 
	 
	\subsection{Additional Results}
	
	\subsubsection{Cost Trials}
	
	Table \ref{TAB:CostCompDetailed} provides detailed results regarding our trials starting at unit costs. 
	
	\begin{table}
		\TABLE
		{Results of price equilibrium computations starting at unit costs under both demand models for ten $1,000$-sample sets. $n$: iterations to termination (maximum is 75); $t$: CPU time (in seconds); ``FO'': First-order conditions satisfied (``S'') or failed (``F''); ``SO'': Second-order conditions satisfied (``S'') or failed (``F''); $\abs{ \vec{p}_* - \vec{p}_*^{\text{FPI}}}$: absolute deviation from equilibrium prices computed by $\bsym{\zeta}$-FPI (in 1980 and 1983 USD). \label{TAB:CostCompDetailed}}
		{\begin{tabular}{cccccccccccccccccccccccccccccccccccccc}
			\\
			\multicolumn{7}{c}{\cite{Boyd80}} && \multicolumn{7}{c}{\cite{Berry95}} \\ \cline{1-7} \cline{9-15} \\
			\\
			\multicolumn{7}{c}{$\bsym{\eta}$-NM} && \multicolumn{7}{c}{$\bsym{\eta}$-NM} \\ \cline{1-7} \cline{9-15}
			&&&& \multicolumn{3}{c}{$\abs{ \vec{p}_* - \vec{p}_*^{\text{FPI}} }$} &&&&&&& \multicolumn{3}{c}{$\abs{ \vec{p}_* - \vec{p}_*^{\text{FPI}} }$} \\ \cline{5-7} \cline{13-15}
		$n$	&	$t$ 		&	FO	&	SO	& min 		& median 		& max 		&	&	$n$	&	$t$		&	FO	&	SO	&	min		&	median	&	max	\\ \cline{1-7} \cline{9-15}
		8	&	77.32	&	S	&	S	&	1.30E-06	&	1.84E-03	&	5.68E+00	&	&	5	&	52.64	&	S	&	S	&	8.97E-05	&	4.20E-02	&	1.16E+02	\\
		75	&	530.51	&	F	&	F	&	6.88E-02	&	1.84E+02	&	6.27E+04	&	&	7	&	65.56	&	S	&	S	&	8.71E-04	&	3.13E-02	&	1.44E+01	\\
		8	&	75.62	&	S	&	S	&	8.15E-05	&	8.01E-03	&	7.61E+00	&	&	5	&	50.67	&	S	&	S	&	1.90E-07	&	1.12E-04	&	1.78E-02	\\
		75	&	508.77	&	F	&	F	&	7.06E-03	&	8.56E+01	&	7.28E+03	&	&	5	&	52.2		&	S	&	S	&	3.29E-06	&	4.13E-03	&	5.47E+00	\\
		13	&	113.66	&	S	&	S	&	1.16E-04	&	8.11E-03	&	7.58E+00	&	&	5	&	52.84	&	S	&	S	&	2.80E-06	&	8.54E-04	&	2.26E+00	\\
		14	&	122.84	&	S	&	S	&	1.95E-06	&	8.54E-03	&	9.80E+00	&	&	5	&	50.47	&	S	&	S	&	6.81E-07	&	5.01E-04	&	3.59E-03	\\
		9	&	86.64	&	S	&	S	&	1.31E-04	&	1.06E-02	&	1.29E+01	&	&	5	&	50.52	&	S	&	S	&	5.36E-08	&	5.27E-04	&	3.88E-03	\\
		7	&	70.62	&	S	&	S	&	5.32E-04	&	1.37E-02	&	1.33E+01	&	&	7	&	63.38	&	S	&	S	&	9.86E-08	&	7.77E-05	&	1.27E-03	\\
		75	&	556.99	&	F	&	F	&	8.66E-02	&	2.77E+01	&	4.52E+04	&	&	5	&	50.8	&	S	&	S	&	8.56E-06	&	1.14E-04	&	1.62E-03	\\
		11	&	100.06	&	S	&	S	&	1.57E-05	&	2.10E-03	&	4.29E-01	&	&	8	&	69.5	&	S	&	S	&	2.07E-06	&	5.85E-04	&	1.64E-02	\\\cline{1-7} \cline{9-15}
		8	&	70.62	&	min	&		&		&		&		&	&	6	&	50.47	&	min	&		&		&		&		\\
		10	&	86.64	&	med	&		&		&		&		&	&	6	&	52.42	&	med	&		&		&		&		\\
		15	&	122.84	&	max	&		&		&		&		&	&	9	&	69.5	&	max	&		&		&		&		\\ \cline{1-7} \cline{9-15}
			\\
			\multicolumn{7}{c}{$\bsym{\zeta}$-NM} && \multicolumn{7}{c}{$\bsym{\zeta}$-NM} \\ \cline{1-7} \cline{9-15}
			&&&& \multicolumn{3}{c}{$\abs{ \vec{p}_* - \vec{p}_*^{\text{FPI}} }$} &&&&&&& \multicolumn{3}{c}{$\abs{ \vec{p}_* - \vec{p}_*^{\text{FPI}} }$} \\ \cline{5-7} \cline{13-15}
		$n$	&	$t$ 	&	FO	&	SO	& min & median & max &	&	$n$	&	$t$	&	FO	&	SO	&	min	&	median	&	max	\\ \cline{1-7} \cline{9-15}
		17	&	125.56	&	S	&	S	&	2.59E-06	&	1.84E-03	&	5.63E+00	&	&	7	&	64.21	&	S	&	S	&	4.21E-05	&	4.39E-02	&	1.22E+02	\\
		9	&	80.35	&	S	&	S	&	4.99E-05	&	1.06E-02	&	2.22E+01	&	&	8	&	70.11	&	S	&	S	&	1.03E-03	&	2.97E-02	&	1.27E+01	\\
		12	&	108.67	&	S	&	S	&	6.47E-05	&	8.01E-03	&	7.61E+00	&	&	29	&	257.25	&	F	&	F	&	3.62E-06	&	5.19E-02	&	2.48E+00	\\
		75	&	507.52	&	F	&	F	&	9.78E-02	&	6.79E+01	&	5.62E+03	&	&	8	&	69.67	&	S	&	S	&	2.36E-04	&	6.41E-03	&	9.58E+00	\\
		75	&	501.52	&	F	&	F	&	7.81E-02	&	2.58E+02	&	1.58E+04	&	&	7	&	65.53	&	S	&	S	&	3.48E-07	&	1.22E-03	&	5.20E-01	\\
		14	&	116.82	&	S	&	S	&	8.12E-06	&	8.55E-03	&	9.80E+00	&	&	10	&	90.16	&	S	&	S	&	7.07E-06	&	6.83E-04	&	3.87E-03	\\
		14	&	119.12	&	S	&	S	&	4.45E-05	&	1.07E-02	&	1.29E+01	&	&	9	&	75.2		&	S	&	S	&	2.27E-07	&	5.92E-04	&	4.42E-03	\\
		19	&	147.41	&	S	&	S	&	3.31E-05	&	1.35E-02	&	1.33E+01	&	&	8	&	72.62	&	S	&	S	&	1.88E-07	&	6.27E-04	&	5.04E-03	\\
		75	&	556.26	&	F	&	F	&	2.32E-03	&	2.43E+01	&	4.51E+04	&	&	8	&	74.91	&	S	&	S	&	1.55E-07	&	4.41E-04	&	3.54E-03	\\
		75	&	508.17	&	F	&	F	&	2.37E-01	&	1.03E+02	&	6.60E+04	&	&	8	&	72.88	&	S	&	S	&	9.80E-06	&	7.09E-04	&	6.63E-03	\\	\\ \cline{1-7} \cline{9-15}
		10	&	80.35	&	min	&		&		&		&		&	&	8	&	64.21	&	min	&		&		&		&		\\
		15	&	117.97	&	med	&		&		&		&		&	&	9	&	72.62	&	med	&		&		&		&		\\
		20	&	147.41	&	max	&		&		&		&		&	&	11	&	90.16	&	max	&		&		&		&		\\ \cline{1-7} \cline{9-15}
		\\
			\multicolumn{4}{c}{$\bsym{\zeta}$-FPI} &&&&& \multicolumn{4}{c}{$\bsym{\zeta}$-FPI} \\ \cline{1-4} \cline{9-12}
		$n$	&	$t$	&	FO	&	SO	&		&		&		&	&	$n$	&	$t$	&	FO	&	SO	&		&		&		\\ \cline{1-4} \cline{9-12}
		24	&	18.07	&	S	&	S	&		&		&		&	&	19	&	24.35	&	S	&	S	&		&		&		\\
		70	&	52.58	&	S	&	S	&		&		&		&	&	18	&	22.58	&	S	&	S	&		&		&		\\
		36	&	27.58	&	S	&	S	&		&		&		&	&	22	&	27.47	&	S	&	S	&		&		&		\\
		29	&	22.02	&	S	&	S	&		&		&		&	&	19	&	23.83	&	S	&	S	&		&		&		\\
		53	&	40.26	&	S	&	S	&		&		&		&	&	19	&	23.9	&	S	&	S	&		&		&		\\
		41	&	31.29	&	S	&	S	&		&		&		&	&	19	&	23.7	&	S	&	S	&		&		&		\\
		39	&	29.74	&	S	&	S	&		&		&		&	&	20	&	24.98	&	S	&	S	&		&		&		\\
		38	&	28.93	&	S	&	S	&		&		&		&	&	23	&	28.62	&	S	&	S	&		&		&		\\
		44	&	33.62	&	S	&	S	&		&		&		&	&	22	&	27.39	&	S	&	S	&		&		&		\\
		23	&	17.37	&	S	&	S	&		&		&		&	&	19	&	23.56	&	S	&	S	&		&		&		\\ \cline{1-4} \cline{9-12}
		23	&	17.37	&	min	&		&		&		&		&	&	18	&	22.58	&	min	&		&		&		&		\\
		38.5	&	29.335	&	med	&		&		&		&		&	&	19	&	24.125	&	med	&		&		&		&		\\
		70	&	52.58	&	max	&		&		&		&		&	&	23	&	28.62	&	max	&		&		&		&		\\ \cline{1-4} \cline{9-12}
			\\
			\\ \cline{1-15}\cline{1-15}
		\end{tabular}}
		{}
	\end{table}
